# Supplementary material for: Localising In-Domain Adaptation of Transformer-Based Biomedical Language Models
Source: arXiv:2212.10422 ancillary file (2023-06-28)

## Supplementary Notes

**Table A1: Details about example drops introduced by the neural machine translation procedure.**

| <b>Dataset</b>    | <b>Type</b> | <b>Original</b> | <b>Translated and Filtered</b> | <b>Dropped</b> | <b>%Drop</b> |
|-------------------|-------------|-----------------|--------------------------------|----------------|--------------|
| BC2GM             | NER         | 24596           | 24341                          | 255            | 1.00%        |
| BC4CHEMD          | NER         | 84355           | 82844                          | 1511           | 1.80%        |
| BC5CDR CDR        | NER         | 28785           | 27554                          | 1231           | 4.30%        |
| BC5CDR DNER       | NER         | 25351           | 24925                          | 426            | 1.70%        |
| BioASQ 4b-factoid | QA          | 2400            | 1871                           | 529            | 22.00%       |
| BioASQ 5b-factoid | QA          | 4153            | 3403                           | 750            | 18.10%       |
| BioASQ 6b-factoid | QA          | 3352            | 2640                           | 712            | 21.20%       |
| BioRED            | RE          | 20419           | 18970                          | 1449           | 0.70%        |
| CHEMPROT          | RE          | 62147           | 61594                          | 553            | 0.90%        |
| NCBI Disease      | NER         | 6892            | 6796                           | 96             | 1.40%        |
| Species-800       | NER         | 3708            | 3696                           | 12             | 0.30%        |

**Table A2: Model configurations details.**

| Model Name                         | Corpus     |            |           | Training Hyperparameters |       |              |              |          | CF Mitigation |      |      |      |      | MLM Performance |        |        |
|------------------------------------|------------|------------|-----------|--------------------------|-------|--------------|--------------|----------|---------------|------|------|------|------|-----------------|--------|--------|
|                                    | Checkpoint | Domain     | Size (GB) | Epochs                   | Batch | Weight Decay | Adam Epsilon | LR       | LLRD          | LF   | ER   | M    | WU   | Loss            | MRR    | PPPL   |
| BaseBIT                            | n.a.       | Generic    | 81        | 3Mstep                   | n.a.  | 1.00E-02     | 1.00E-06     | 5.00E-05 | n.a.          | n.a. | n.a. | n.a. | n.a. | n.a.            | 0.3429 | 2.3744 |
| BioBIT <sub>XS</sub>               | Base       | Biomedical | 0.1       | 3                        | n.a.  | 1.00E-02     | 1.00E-06     | 5.00E-05 | n.a.          | n.a. | n.a. | n.a. | n.a. | 1.204           | 0.3432 | 2.4531 |
| BioBIT <sub>S</sub>                | Base       | Biomedical | 0.3       | 3                        | n.a.  | 1.00E-02     | 1.00E-06     | 5.00E-05 | n.a.          | n.a. | n.a. | n.a. | n.a. | 1.08            | 0.3536 | 2.5917 |
| BioBIT <sub>M</sub>                | Base       | Biomedical | 1         | 3                        | n.a.  | 1.00E-02     | 1.00E-06     | 5.00E-05 | n.a.          | n.a. | n.a. | n.a. | n.a. | 0.996           | 0.3517 | 2.8370 |
| BioBIT <sub>L</sub>                | Base       | Biomedical | 28        | 10                       | n.a.  | 1.00E-02     | 1.00E-06     | 5.00E-05 | n.a.          | n.a. | n.a. | n.a. | n.a. | 0.7             | 0.3829 | 3.3504 |
| MedBIT                             | BioBIT_L   | Medical    | 0.1       | 10                       | 16    | 1.00E-02     | 1.00E-06     | 5.00E-05 | n.a.          | n.a. | n.a. | n.a. | n.a. | 1.922           | 0.3651 | 2.3893 |
| MedBIT <sub>R0</sub>               | BioBIT_L   | Medical    | 0.1       | 3                        | 16    | 1.00E-02     | 1.00E-06     | 5.00E-05 | 0.9           | n.a. | 100  | n.a. | n.a. | 1.375           | 0.3761 | 2.2527 |
| MedBIT <sub>R1</sub>               | BioBIT_L   | Medical    | 0.1       | 3                        | 16    | 1.00E-02     | 1.00E-06     | 5.00E-05 | 0.9           | n.a. | 100  | 0.9  | n.a. | 1.375           | 0.3731 | 2.3145 |
| MedBIT <sub>R2</sub>               | BioBIT_L   | Medical    | 0.1       | 3                        | 16    | 1.00E-02     | 1.00E-06     | 5.00E-05 | 0.9           | n.a. | n.a. | 0.9  | n.a. | 1.361           | 0.3771 | 2.3019 |
| MedBIT <sub>R3</sub>               | BioBIT_L   | Medical    | 0.1       | 7                        | 16    | 1.00E-02     | 1.00E-06     | 5.00E-05 | 0.9           | n.a. | n.a. | 0.9  | 0.02 | 1.329           | 0.3776 | 2.2792 |
| MedBIT <sub>RF</sub>               | BioBIT_L   | Medical    | 0.1       | 10                       | 16    | 1.00E-02     | 1.00E-06     | 5.00E-05 | n.a.          | 6    | n.a. | n.a. | n.a. | 2.024           | 0.3704 | 2.4033 |
| MedBIT <sub>OR</sub>               | Base       | Medical    | 0.1       | 7                        | 16    | 1.00E-02     | 1.00E-06     | 5.00E-05 | 0.9           | n.a. | n.a. | 0.9  | 0.02 | 1.312           | 0.3498 | 2.2030 |
| MedBIT <sub>R3</sub> <sup>+</sup>  | BioBIT_L   | Medical    | 0.2       | 7                        | 16    | 1.00E-02     | 1.00E-06     | 5.00E-05 | 0.9           | n.a. | n.a. | 0.9  | 0.02 | 1.321           | 0.3750 | 2.1677 |
| MedBIT <sub>R3f</sub>              | BioBIT_L   | Medical    | 0.1       | 10                       | 16    | 1.00E-02     | 1.00E-06     | 3.00E-05 | 0.95          | n.a. | n.a. | 0.9  | 0.02 | 1.521           | 0.3781 | 2.3808 |
| MedBIT <sub>R4</sub>               | BioBIT_L   | Medical    | 0.1       | 10                       | 16    | 1.00E-02     | 1.00E-06     | 3.00E-05 | 0.9           | n.a. | 50   | n.a. | n.a. | n.a.            | n.a.   | n.a.   |
| MedBIT <sub>R5</sub>               | BioBIT_L   | Medical    | 0.1       | 10                       | 16    | 1.00E-02     | 1.00E-06     | 3.00E-05 | 0.9           | n.a. | 10   | n.a. | n.a. | n.a.            | n.a.   | n.a.   |
| MedBIT <sub>R6</sub>               | BioBIT_L   | Medical    | 0.1       | 10                       | 16    | 1.00E-02     | 1.00E-06     | 3.00E-05 | 0.9           | n.a. | 25   | n.a. | n.a. | n.a.            | n.a.   | n.a.   |
| MedBIT <sub>R7</sub>               | BioBIT_L   | Medical    | 0.1       | 10                       | 16    | 1.00E-02     | 1.00E-06     | 3.00E-05 | 0.9           | 6    | 50   | n.a. | n.a. | n.a.            | n.a.   | n.a.   |
| MedBIT <sub>R8</sub>               | BioBIT_L   | Medical    | 0.1       | 10                       | 16    | 1.00E-02     | 1.00E-06     | 3.00E-05 | 0.9           | 3    | 50   | n.a. | n.a. | n.a.            | n.a.   | n.a.   |
| MedBIT <sub>R9</sub>               | BioBIT_L   | Medical    | 0.1       | 10                       | 16    | 1.00E-02     | 1.00E-06     | 3.00E-05 | 0.8           | n.a. | 50   | n.a. | n.a. | n.a.            | n.a.   | n.a.   |
| MedBIT <sub>R10</sub>              | BioBIT_L   | Medical    | 0.1       | 10                       | 16    | 1.00E-02     | 1.00E-06     | 3.00E-05 | 0.95          | n.a. | 50   | n.a. | n.a. | n.a.            | n.a.   | n.a.   |
| MedBIT <sub>R11</sub>              | BioBIT_L   | Medical    | 0.1       | 10                       | 16    | 1.00E-02     | 1.00E-06     | 3.00E-05 | 0.99          | n.a. | 50   | n.a. | n.a. | n.a.            | n.a.   | n.a.   |
| MedBIT <sub>R12</sub>              | BioBIT_L   | Medical    | 0.1       | 10                       | 16    | 2.00E-02     | 1.00E-06     | 3.00E-05 | 0.95          | n.a. | 50   | n.a. | n.a. | n.a.            | n.a.   | n.a.   |
| MedBIT <sub>R12</sub> <sup>+</sup> | BioBIT_L   | Medical    | 0.2       | 10                       | 16    | 2.00E-02     | 1.00E-06     | 3.00E-05 | 0.95          | n.a. | 50   | n.a. | n.a. | n.a.            | 0.3844 | 2.0163 |

**Table A3: Model nomenclature summary.**

| Model Name                        | Description                                                                                                                                                                                                                                                                                                                                                   |
|-----------------------------------|---------------------------------------------------------------------------------------------------------------------------------------------------------------------------------------------------------------------------------------------------------------------------------------------------------------------------------------------------------------|
| BERT <sub>Multi</sub>             | Multilingual version of BERT, trained on multiple generic corpora from different languages, Italian included.                                                                                                                                                                                                                                                 |
| BaseBIT                           | The baseline model, trained on generic Italian corpora.                                                                                                                                                                                                                                                                                                       |
| BioBIT <sub>XS/S/M/L</sub>        | The biomedical model, trained on biomedical corpus (i.e., PubMed abstracts). The subscript nomenclature indicates the size of the training corpus (XS=smaller, L=larger=whole dataset).                                                                                                                                                                       |
| MedBIT <sub>Rn</sub>              | The biomedical model, subsequently trained on a collection of Italian medical textbooks with different CF mitigation techniques ("R"="regularized"). The increasing subscript number, here referred to as "n", is used to differentiate the various configurations tested. Details about such configurations can be found in table A2 of Supplementary Notes. |
| MedBIT <sub>OR</sub>              | The model trained directly on the Italian medical textbooks collection, skipping the BioBIT checkpoint ("O"="original") and using CF mitigation techniques.                                                                                                                                                                                                   |
| MedBIT <sub>Rn</sub> <sup>+</sup> | Like MedBIT <sub>Rn</sub> , but the medical textbooks corpora it is trained on has been augmented with web scraped texts from Italian medical sources.                                                                                                                                                                                                        |

**Table A4: Corpora comparison in terms of unique words, sentences, words and average sentence length.**

|                                 | PRE-<br>TRAINING<br>(Reference) | BC2GM                | BC4CHE<br>MD          | BC5CDR<br>_CDR       | BC5CDR<br>_DNER       | NCBI_DI<br>SEASE     | SPECIES<br>_800      | BIOASQ<br>_4B       | BIOASQ<br>_5B        | BIOASQ<br>_6B         | BIORED              | CHEMD<br>NER         |
|---------------------------------|---------------------------------|----------------------|-----------------------|----------------------|-----------------------|----------------------|----------------------|---------------------|----------------------|-----------------------|---------------------|----------------------|
| Unique<br>words                 | 141.3×10 <sup>4</sup>           | 1.7×10 <sup>4</sup>  | 5.5×10 <sup>4</sup>   | 1.0×10 <sup>4</sup>  | 11.5×10 <sup>4</sup>  | 0.9×10 <sup>4</sup>  | 1.8×10 <sup>4</sup>  | 0.7×10 <sup>4</sup> | 0.9×10 <sup>4</sup>  | 1.0×10 <sup>4</sup>   | 5.0×10 <sup>4</sup> | 1.5×10 <sup>4</sup>  |
| Sentences                       | 18937.5×10 <sup>4</sup>         | 0.5×10 <sup>4</sup>  | 5.1×10 <sup>4</sup>   | 0.5×10 <sup>4</sup>  | 17.8×10 <sup>4</sup>  | 0.5×10 <sup>4</sup>  | 0.8×10 <sup>4</sup>  | 0.2×10 <sup>4</sup> | 0.4×10 <sup>4</sup>  | 0.3×10 <sup>4</sup>   | 0.1×10 <sup>4</sup> | 0.6×10 <sup>4</sup>  |
| Words                           | 486769×10 <sup>4</sup>          | 14.2×10 <sup>4</sup> | 151.0×10 <sup>4</sup> | 11.6×10 <sup>4</sup> | 537.3×10 <sup>4</sup> | 13.4×10 <sup>4</sup> | 21.0×10 <sup>4</sup> | 7.4×10 <sup>4</sup> | 13.0×10 <sup>4</sup> | 112.0×10 <sup>4</sup> | 3.2×10 <sup>4</sup> | 18.1×10 <sup>4</sup> |
| Sentence<br>Length<br>(Average) | 25.7                            | 29.1                 | 29.7                  | 24.9                 | 30.2                  | 24.9                 | 25.6                 | 39.3                | 34.6                 | 36.4                  | 28.6                | 28.8                 |

**Table A5: Downstream corpora comparison in terms of keyness with reference to the pretraining corpus. The table reports the words of the reference corpus with the highest normalized frequency difference with the target corpora. The effect size is calculated in term of log-odds and outliers have been removed.**

| rank | BC2GM                  | BC4CHEMD                      | BC5CDR_CDR             | BC5CDR_DNER            | NCBI_DISEASE              | SPECIES_800            |
|------|------------------------|-------------------------------|------------------------|------------------------|---------------------------|------------------------|
| 1    | encephalopathy-typical | encephalopathy-typical        | encephalopathy-typical | encephalopathy-typical | encephalopathy-typical    | encephalopathy-typical |
| 2    | 347253                 | 18 mj                         | vectec                 | 96                     | n-acetylphenylalanylamide | pser254                |
| 3    | 60422                  | 15094 nm                      | ci = 989-997           | chame-ntd              | -9310                     | socs3cko               |
| 4    | ctv_lob                | sub-micron-diameter           | ci = 793-809           | chame-ntd-gc-fid       | chicken-campylobacter     | calluna-plants         |
| 5    | ctv_fat                | non-transformational          | ci = 892-910           | normal-rbcs            | *biology*                 | calluna-heathlands     |
| 6    | ptw-verisoft           | smf-capillary-smf             | ci = 882-899           | synchronized-pressing  | recognition/prevention    | ii-3301                |
| 7    | mir-106-related        | 18 mj                         | pig-z                  | lifelong-rl            | 205137                    | 640f/815r              |
| 8    | parg527gln             | 35 kw                         | exposure/adherence     | manhattan-based        | gyrobifastigia            | pthr314                |
| 9    | diacylglyceroldag      | 4 mm×4 mm                     | rrchl                  | 551±151                | isometric-isothermal      | pser265                |
| 10   | rs76999397             | phase-shift-amplified         | otherized              | tc_24h_cn              | $\beta = -0082$           | neurons-sympathetic    |
| 11   | ± 108                  | -30 dbm                       | clonidine-only         | ms4a6                  | d*20                      | n = 605                |
| 12   | smoker/smokeless       | dimethylcyclodextrin          | 323-427                | ms4a15                 | $\delta d*20$             | c305g > a              |
| 13   | koa-associated         | fs-lst                        | $\beta = -0082$        | positivefp             | instrumentarium           | co-water               |
| 14   | ≤8 months              | zfh <sub>3</sub> -b           | dwhd                   | chiasm-evoked          | clinicaladministrative    | polyphenol-embedded    |
| 15   | 182-1091               | csh <sub>5</sub> <sup>-</sup> | -9310                  | mtc/s                  | phenol-a                  | 25 t                   |
| 16   | isrctn53778569         | ymsmw                         | chicken-campylobacter  | hd                     | 7.34                      | deoxopinguisone        |
| 17   | rs189013166            | 702 nm                        | generatehope           | aminosilica/graphene   | dwhd                      | no-proteinuria         |
| 18   | rs199772854            | au25-xagxsr18                 | m = 2086               | diisophthalic          | 323-427                   | igf-ii/igf-ir/mek/erk  |
| 19   | otherized              | cls-mr                        | recognition/prevention | non-free-range         | 861 ml                    | peri-operating         |
| 20   | trk-targeting          | parent/high                   | parg527gln             | m377i                  | ci = 989-997              | clinicaladministrative |

[Continuing Table A5]

| rank | BIOASQ_4B              | BIOASQ_5B              | BIOASQ_6B              | BIORED                 | CHEMDNER                      |
|------|------------------------|------------------------|------------------------|------------------------|-------------------------------|
| 1    | encephalopathy-typical | encephalopathy-typical | encephalopathy-typical | encephalopathy-typical | encephalopathy-typical        |
| 2    | exposure/adherence     | ci = 882-899           | vectec                 | rrchl                  | d*20                          |
| 3    | generatehope           | m = 2086               | ci = 989-997           | ci = 793-809           | *biology*                     |
| 4    | ci = 989-997           | otherized              | ci = 793-809           | ci = 892-910           | recognition/prevention        |
| 5    | ci = 793-809           | generatehope           | ci = 892-910           | ci = 882-899           | 205137                        |
| 6    | ci = 892-910           | ci = 989-997           | ci = 882-899           | pig-z                  | gyrobifastigia                |
| 7    | ci = 882-899           | ci = 793-809           | pig-z                  | exposure/adherence     | n-<br>acetylphenylalanylamide |
| 8    | pig-z                  | ci = 892-910           | exposure/adherence     | vectec                 | isometric-isothermal          |
| 9    | vectec                 | pig-z                  | rrchl                  | clonidine-only         | δd*20                         |
| 10   | m = 2086               | 182-1091               | otherized              | generatehope           | -9310                         |
| 11   | rrchl                  | exposure/adherence     | clonidine-only         | 323-427                | instrumentarium               |
| 12   | clonidine-only         | vectec                 | 323-427                | β = -0082              | clinicaladministrative        |
| 13   | 323-427                | rrchl                  | β = -0082              | dwhd                   | phenol-a                      |
| 14   | β = -0082              | clonidine-only         | dwhd                   | -9310                  | 7.34                          |
| 15   | dwhd                   | 323-427                | -9310                  | chicken-campylobacter  | pkh2-transfected              |
| 16   | -9310                  | β = -0082              | chicken-campylobacter  | *biology*              | 861 ml                        |
| 17   | otherized              | isrctn53778569         | generatehope           | ci = 989-997           | chicken-campylobacter         |
| 18   | isrctn53778569         | ≤8 months              | m = 2086               | otherized              | dwhd                          |
| 19   | *biology*              | -9310                  | recognition/prevention | 205137                 | usp14-/-                      |
| 20   | mir-106-related        | ctv_fat                | parg527gln             | 347253                 | ci = 892-910                  |

**Figure A1: Overlap between the top K most frequent keywords of each downstream corpus compared with the pretraining one.**

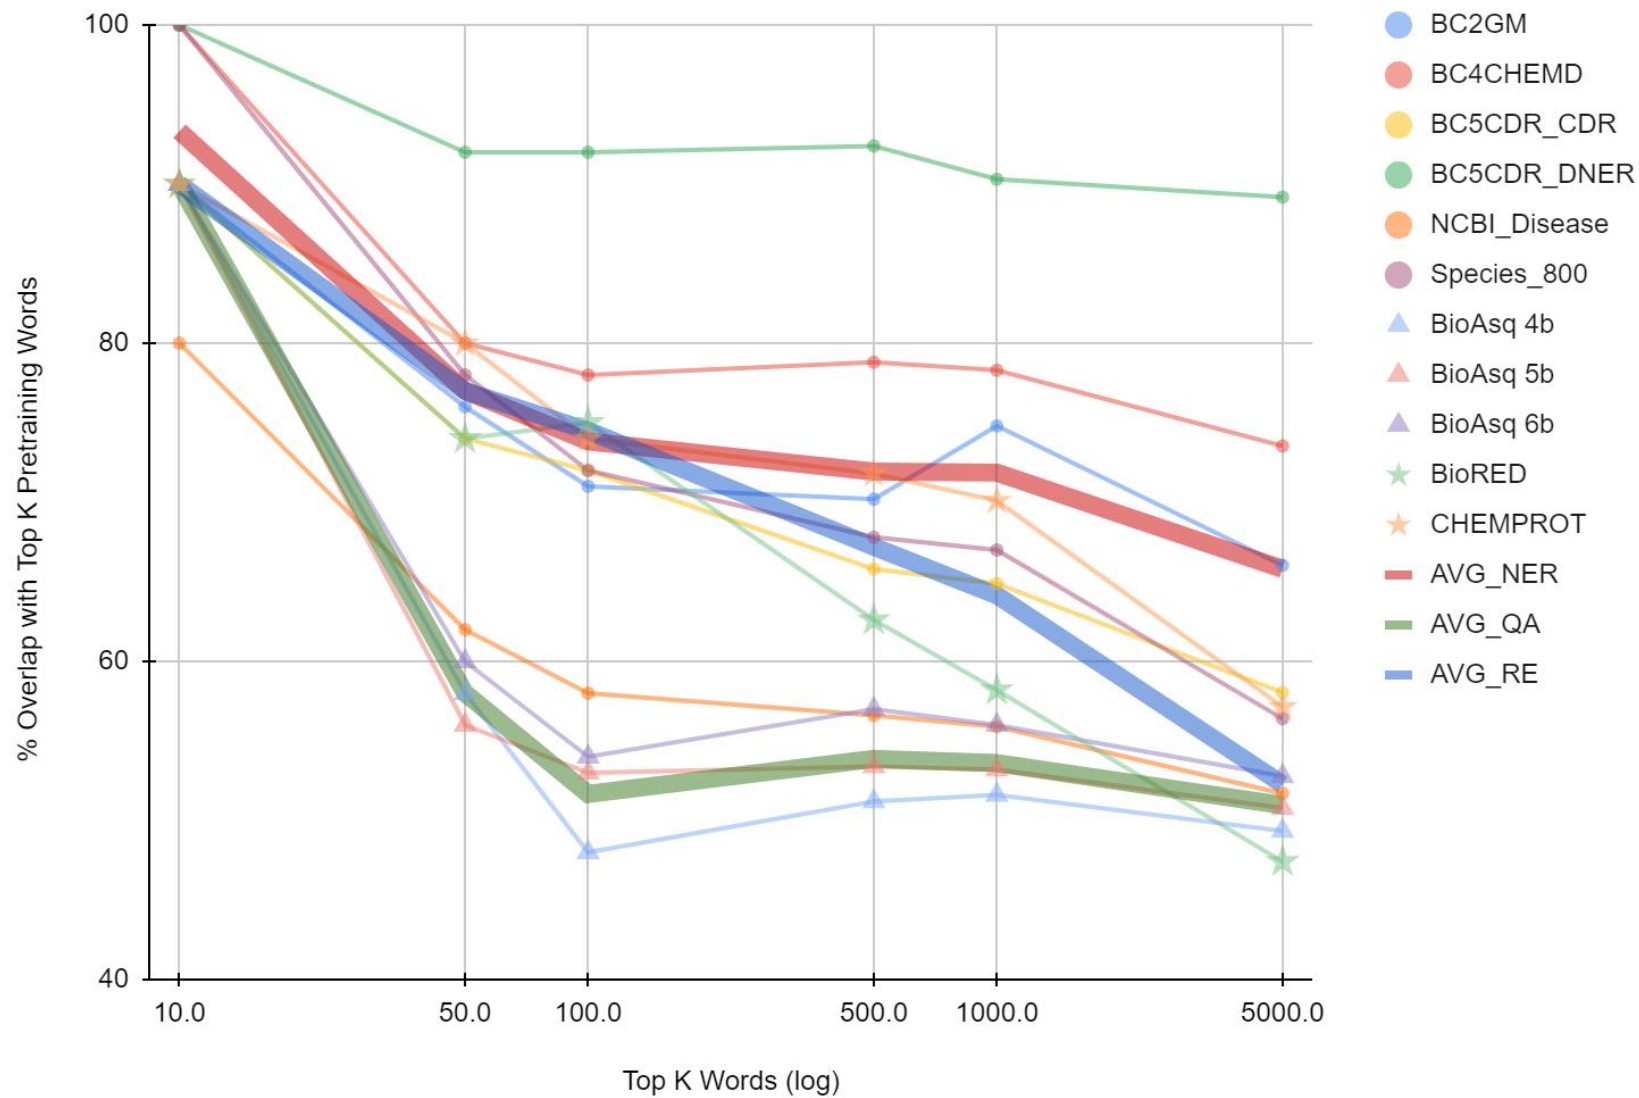

Figure A2: Topic distribution for MLM Dataset and Textbook Corpus.

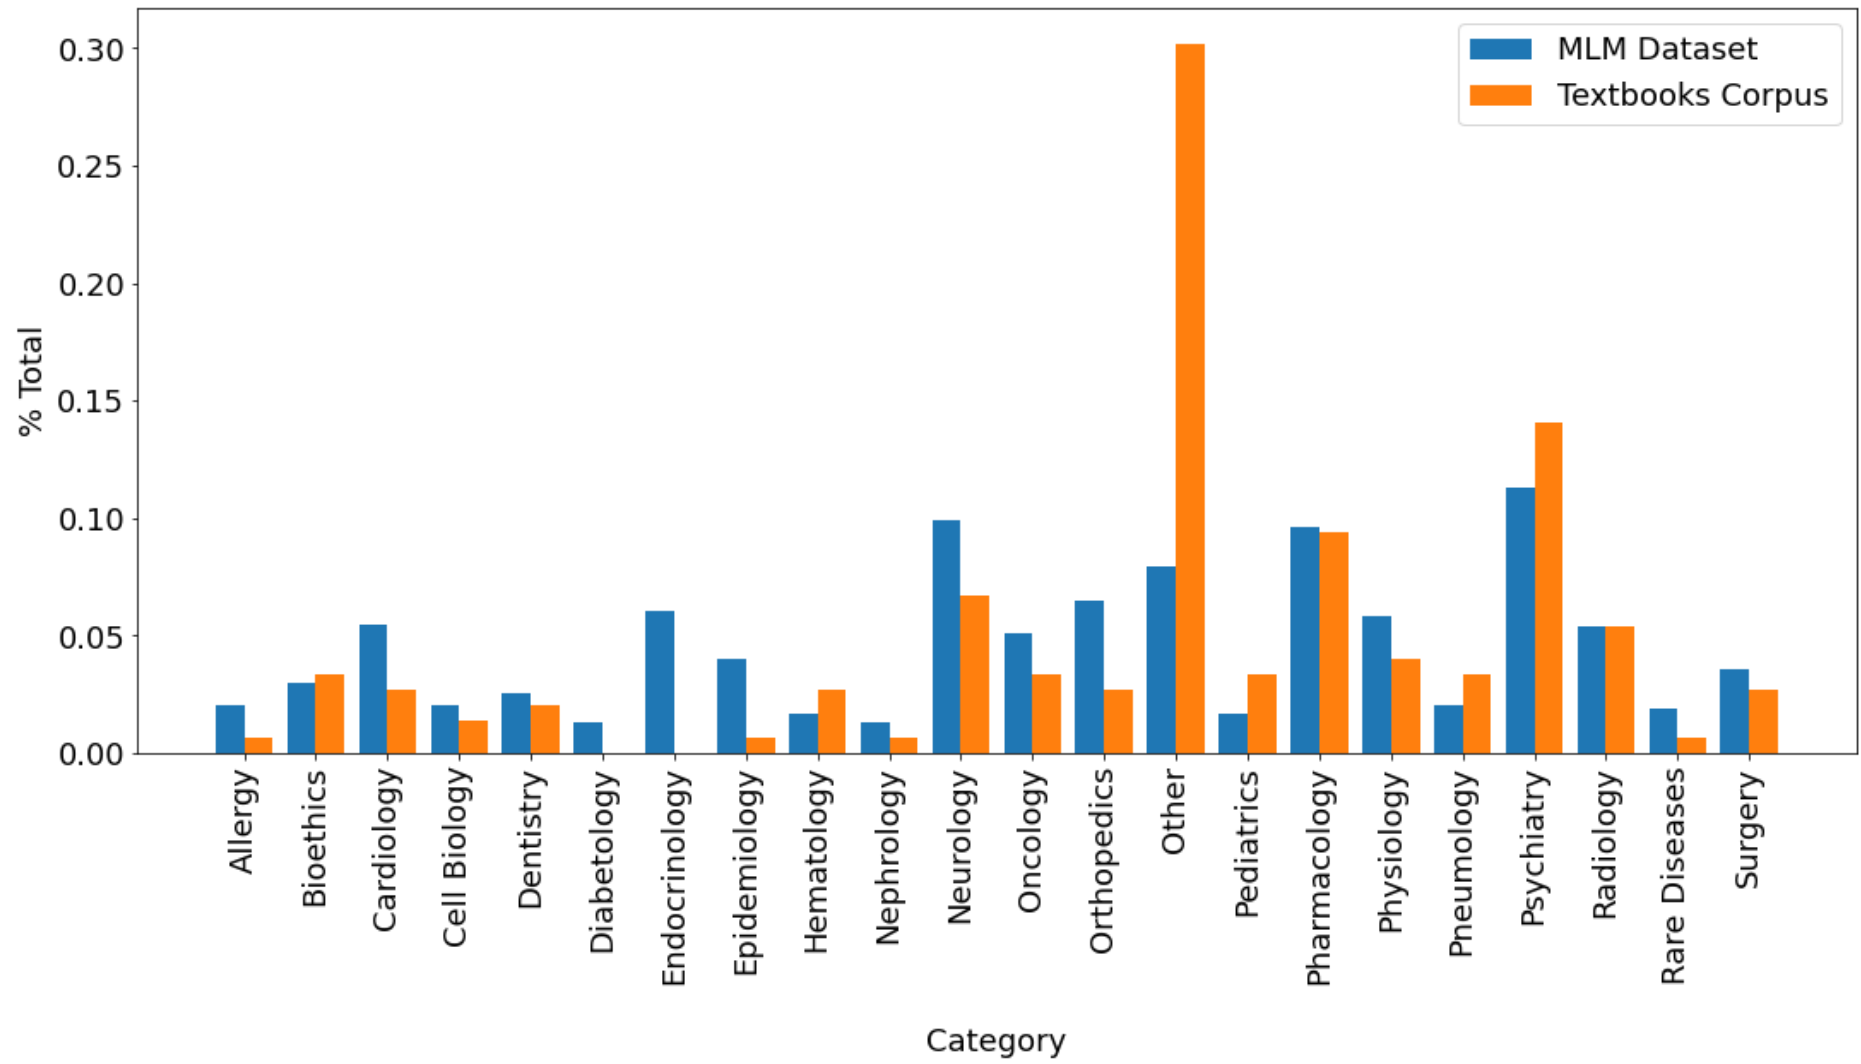

Supplement: Supplementary file 1 [file supplementary_notes_updated.pdf]
